# Supplementary material for: Imaging ultrafast dynamical diffraction wavefronts in strained Si with coherent X-rays
Source: arXiv:2012.08893 source file (2021-10-11)
Supplement: Supplementary file 1 [file SM.pdf]

# Supplementary Information: Imaging ultrafast dynamical diffraction wavefronts in strained Si with coherent X-rays


Angel Rodriguez-Fernandez,[1] Ana Diaz,[2] Anand H. S. Iyer,[3] Mariana Verezhak,[2] Klaus Wakonig,[2] Magnus H. Colliander,[3] and Dina Carbone[4]

[1] *European X-ray Free Electron Laser GmbH, Schenefeld, DE-22986.*[*]
[2] *Paul Scherrer Institute, Forschungsstrasse 111, Villigen. PSI CH-5232*
[3] *Department of Physics, Chalmers University of Technology, Gothenburg SE-41296*
[4] *MAX IV Laboratory, Lund University, Lund, SE-22199.*



(Dated: October 11, 2021)


## I. SUPPLEMENTARY MATERIAL

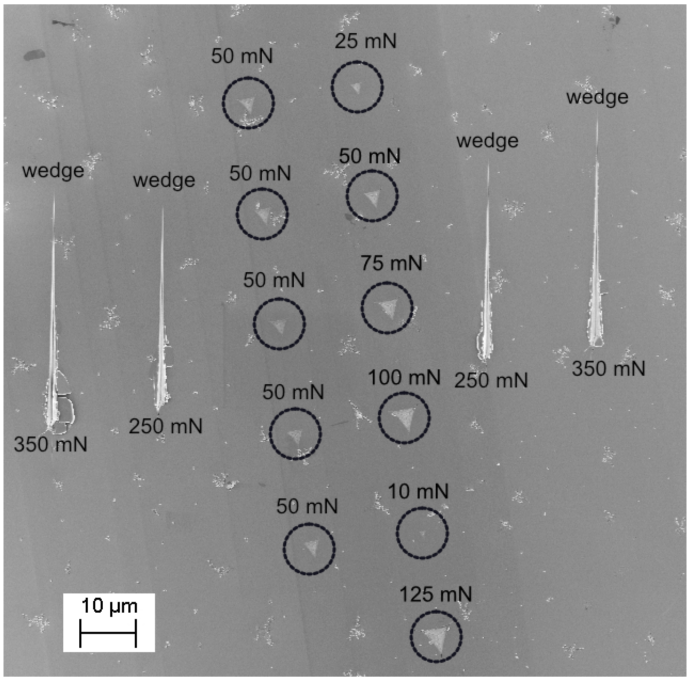


FIG. S1. Map of the indentation performed onto a Si 100 μm thick crystal using an Alemnis in-situ nanoindenter in a Zeiss Leo Ultra 55 FEG SEM. The indentations were carried out using a diamond Berkovich tip with a half angle of 65.3° and leaving 20 μm in between indents. Four long lines were performed to mark the area for an easy location of the nano-indents via optical microscope. Two lines of indentations, one with constant load of 50 mN and a second with a varying load from 10 to 125 mN, were performed. The indentation depth ranged from 200 to 1100 nm and the size of the resulting indents was in the range 1.4 to 5.2 μm.


* angel.rodriguez-fernandez@xfel.eu

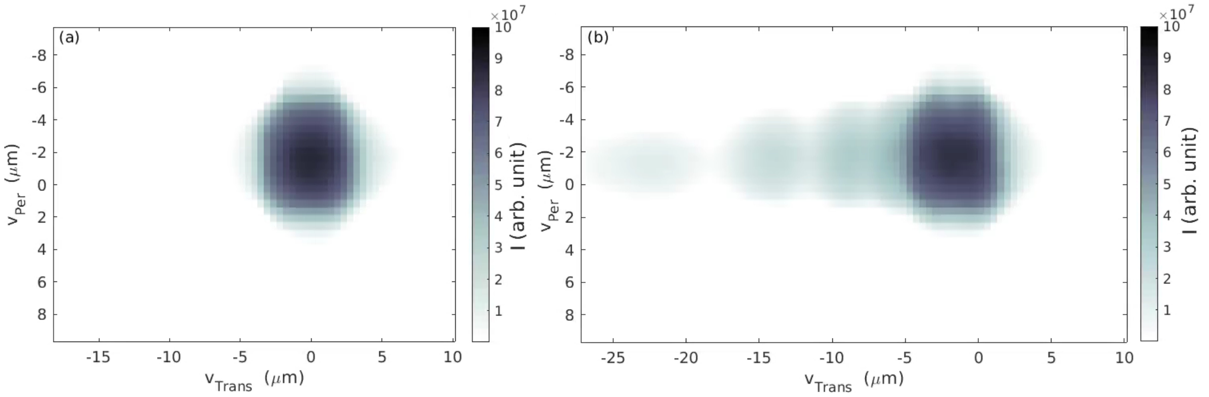


FIG. S2. Scanning transmission X-ray microscopy (STXM) maps of the FD from a 100 µm thick strain-free Si(001) crystal, collected using the tele-ptychography setup, with the pinhole as the scanning probe, (a) with the Si crystal out of diffraction conditions and (b) at the Si(111) Laue diffraction condition at 8 keV. The maps are produced combining the data from several overlapping measurements, as described in the main text. The resolution, given by the convolution between the pinhole size and the distance between two adjacent measurement positions, is 3 µm.

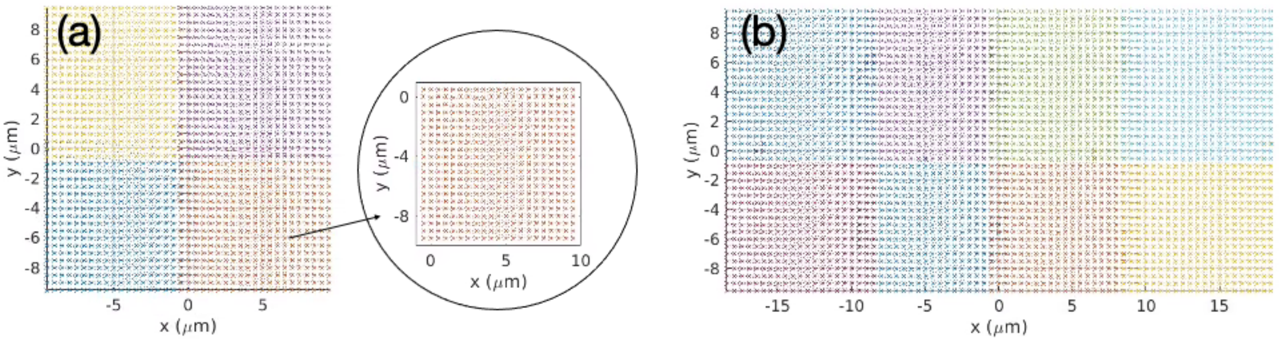


FIG. S3. Position of the scans for the strain-free samples used in the reconstruction [41], (a) outside of the diffraction condition and (b) at the diffraction condition —where the echoes are observed. Each color area refers to a different scan region. The inset represent one single scan inside the collection, and the dots indicate the position of each point of the map.

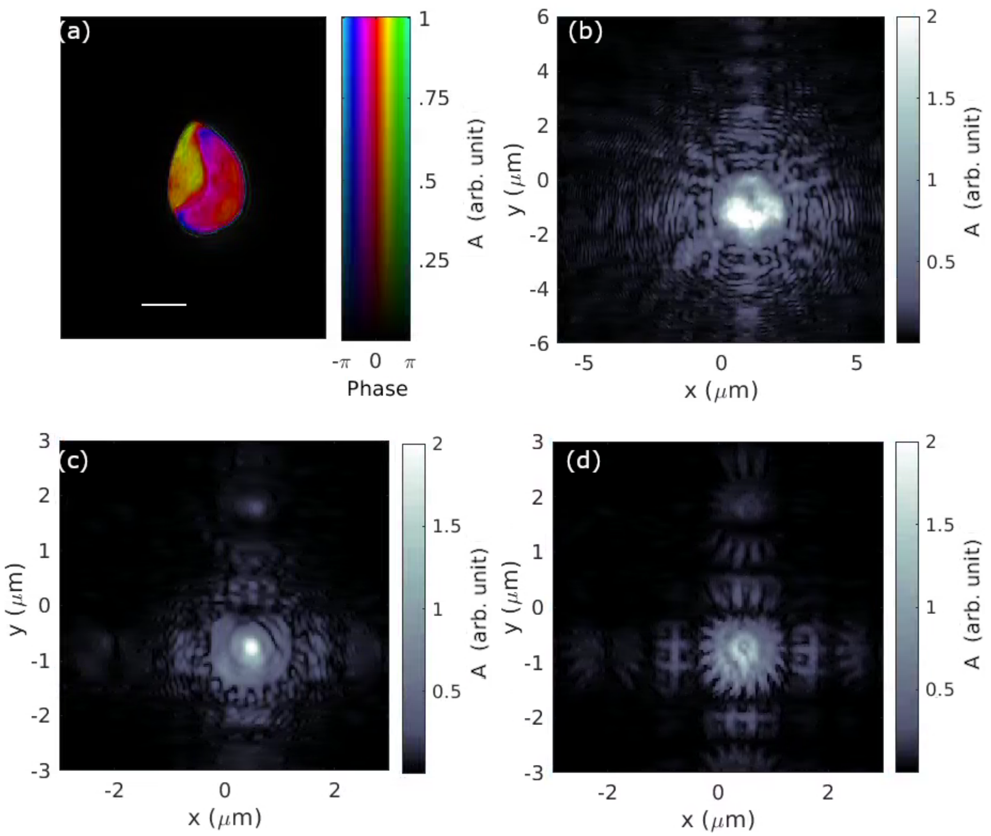


FIG. S4. (a) Reconstruction of the pinhole [29] from a tele-ptychography measurement of the beam transmitted through the NanoMAX standard sample, a pattern of flowers produced with lithography on 500 µm thick diamond window with a 200 nm thin layer of W (U. Vogt et al., International Society for Optics and Photonics (SPIE, 2017) pp. 24 – 30), located 200 µm upstream the KB focus. The color represents the phase, and the intensity represents the amplitude. The white line represents the scale of 2 µm in the pinhole reconstruction. The pinhole is not a perfect circle due to the method of production. The walls of the pinhole have different thickness, that generate the changes in the reconstructed phase. Moreover, residual organic material still present from the fabrication process, and impossible to remove without damaging the pinhole, can be responsible for the phase variation in the middle. The same pinhole has been used in other experiments at other facilities providing identical results, as presented in the supplementary information of [32]. (b) Reconstruction of the transmitted beam amplitude at the pinhole position, 5 mm downstream from the KB focus. (c) Amplitude of the reconstructed wave-front propagated to the KB focus. (d) Amplitude of the reconstructed wave-front propagated to the sample plane 500 µm upstream the KB focus.

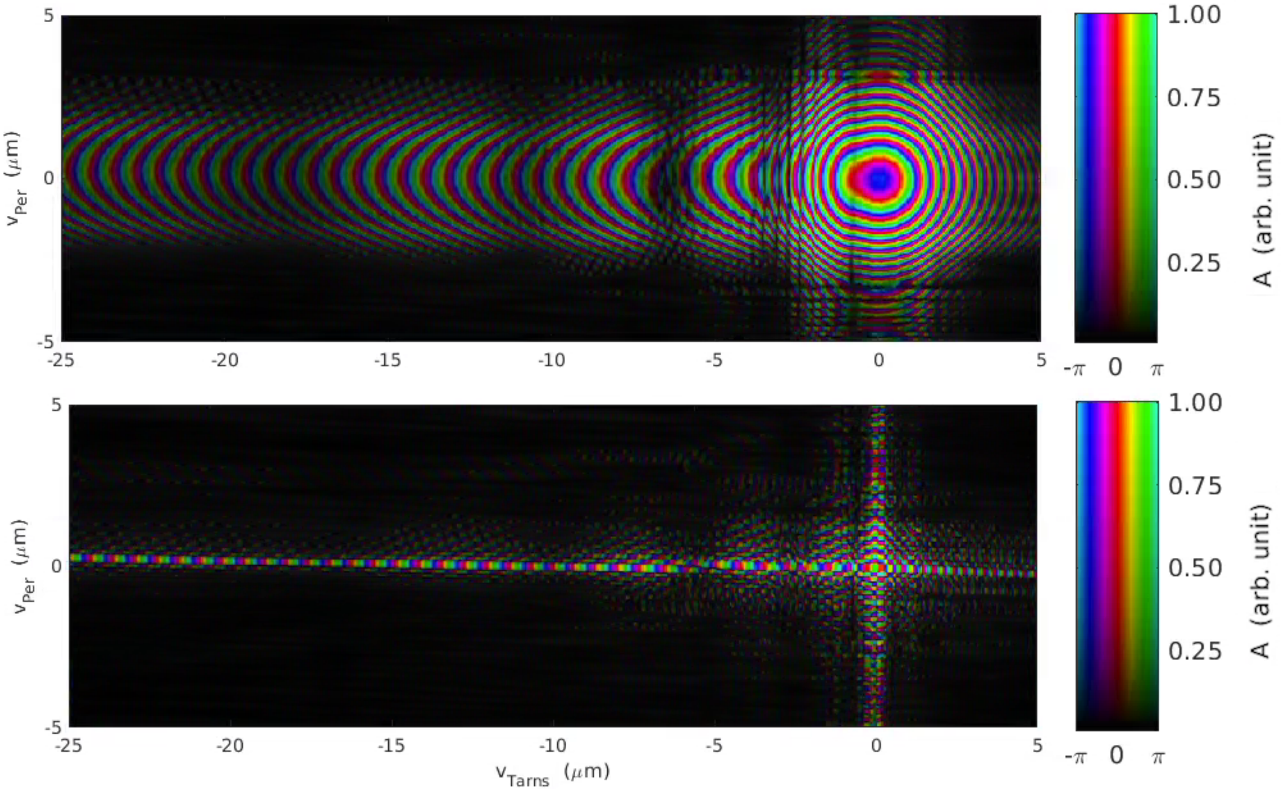


FIG. S5. Reconstruction of the wave front phase and amplitude shown as hue and brightness of the color-map, for the Si(111) asymmetric Laue diffraction condition for the strain-free Si sample at diffraction condition. (Top) At the pinhole location and (bottom) propagated to the sample plane, that coincides with the beam focus.

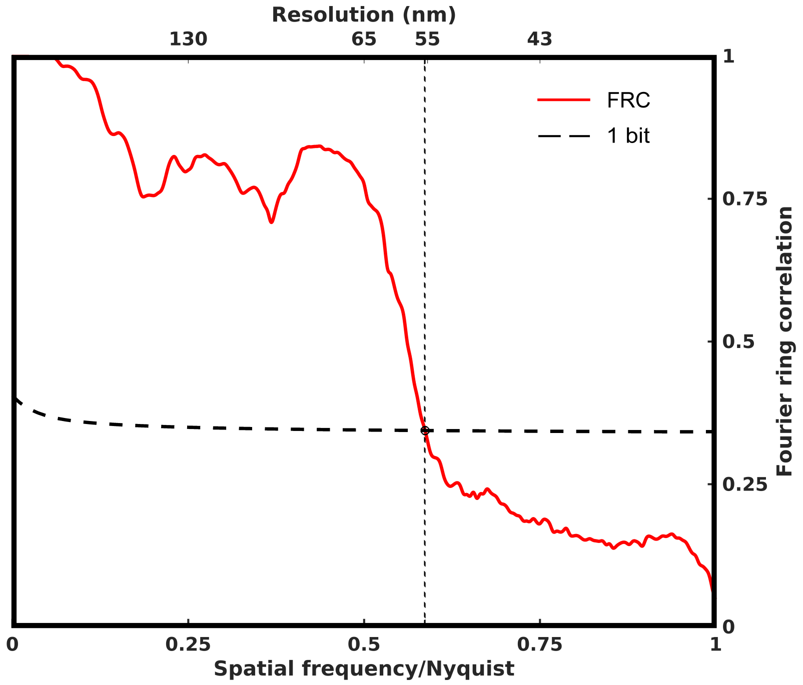


FIG. S6. Fourier ring correlation, following the work by van Heel and Schatz [42], of two ptychographic reconstructions from independent scans of the forward beam out-of-diffraction conditions. The Fourier ring correlation crosses the spatial frequency at a

resolution value of 55 nm.

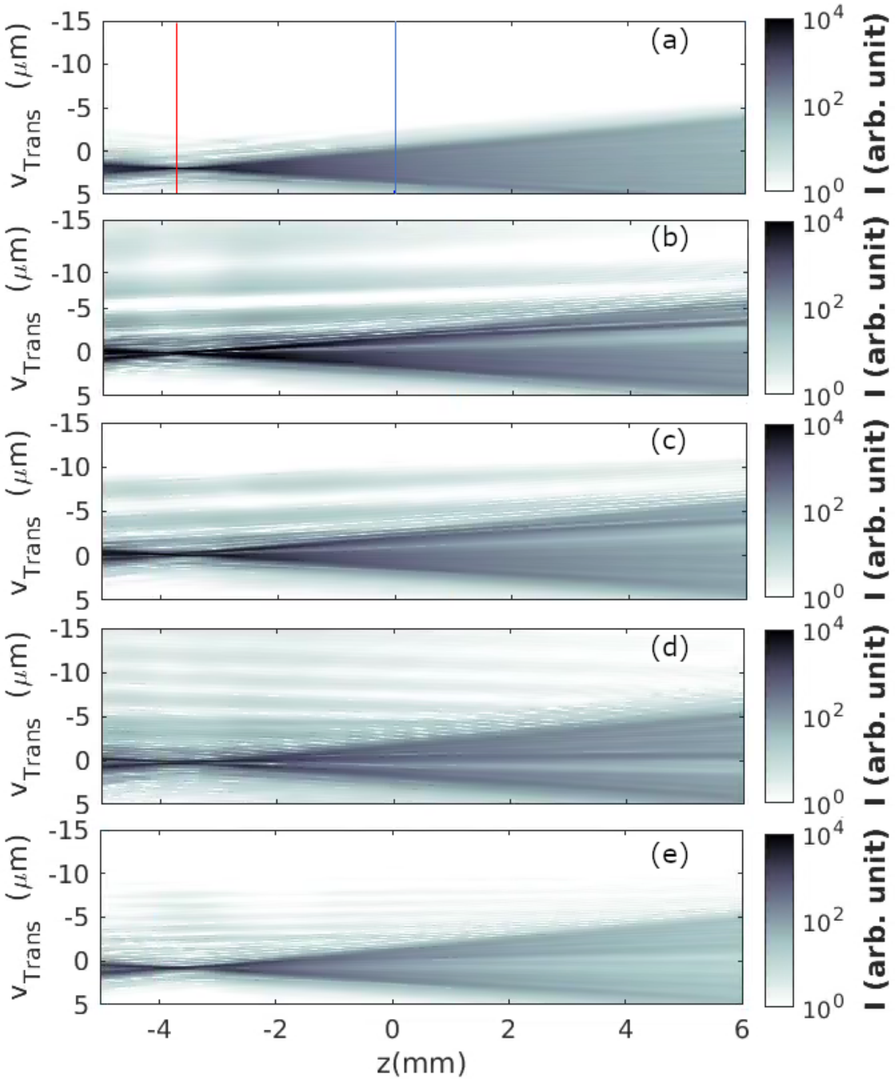


FIG. S7. Map of the reconstructed diffracted intensities along the beam propagation direction in the x-z plane measured on the strain-free Si sample (a) an degree away and (b) at the asymmetric (111) Laue diffraction geometry. Similar maps measured on the indented samples at the asymmetric (111) Laue diffraction geometry (c) 1 mm away from the indented area, (d) on a nano-indent with a 25 mN load and (e) on a nano-indent with a 75 mN load. The native divergence of the focused beam is visible in the incident and transmitted beams, but is not preserved in the echoes. In (a) the red line represents the position of the Si wafer, that coincides with the focus of the KB-mirrors; the blue line represents the position of the pinhole used as analyzer. In this plane the reconstructions are performed.

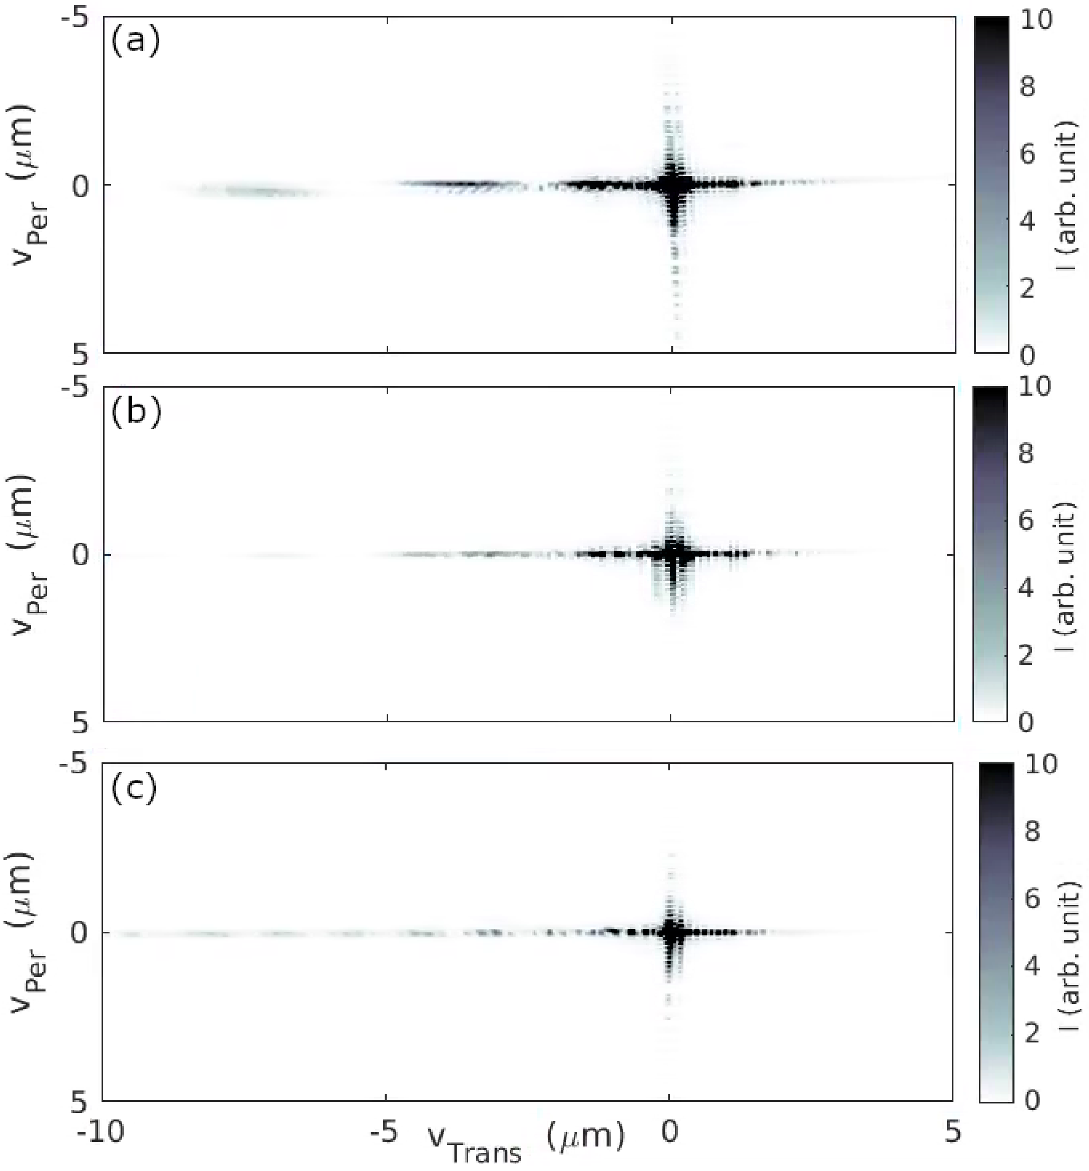


FIG. S8. Maps of the forward diffraction intensities measured with tele-ptychography and propagated to the sample (focus) plane for the indented sample at the asymmetric (111) Laue diffraction geometry, at three positions along the surface with different indentation loads: (a) 1 mm away from the indentation area, (b) 25 mN load and (c) 75 mN load.

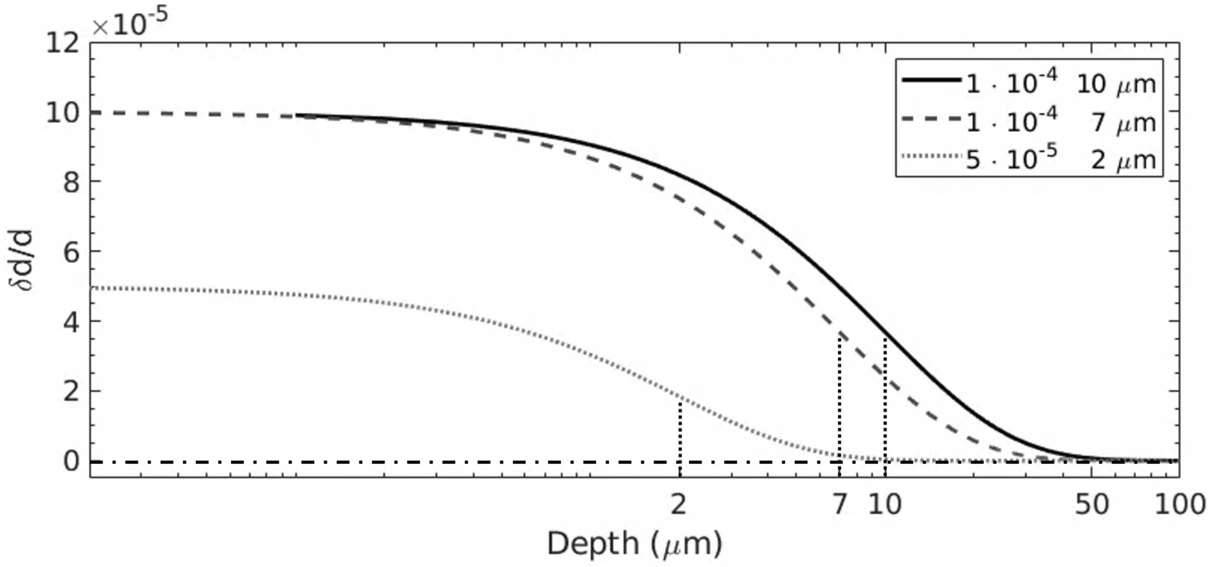


FIG. S9. Strain profiles used in the simulations performed using the dynamical diffraction theory. The strain profiles follow a inverse exponential relation. Three profiles are presented with different surface values of strain $\delta$d/d: (line) $5 \cdot 10^{-5}$, (dot line) $10^{-4}$ and (dash line) $10^{-4}$. The profiles extend over different decay lengths of 10, 7 and 2 µm, respectively.

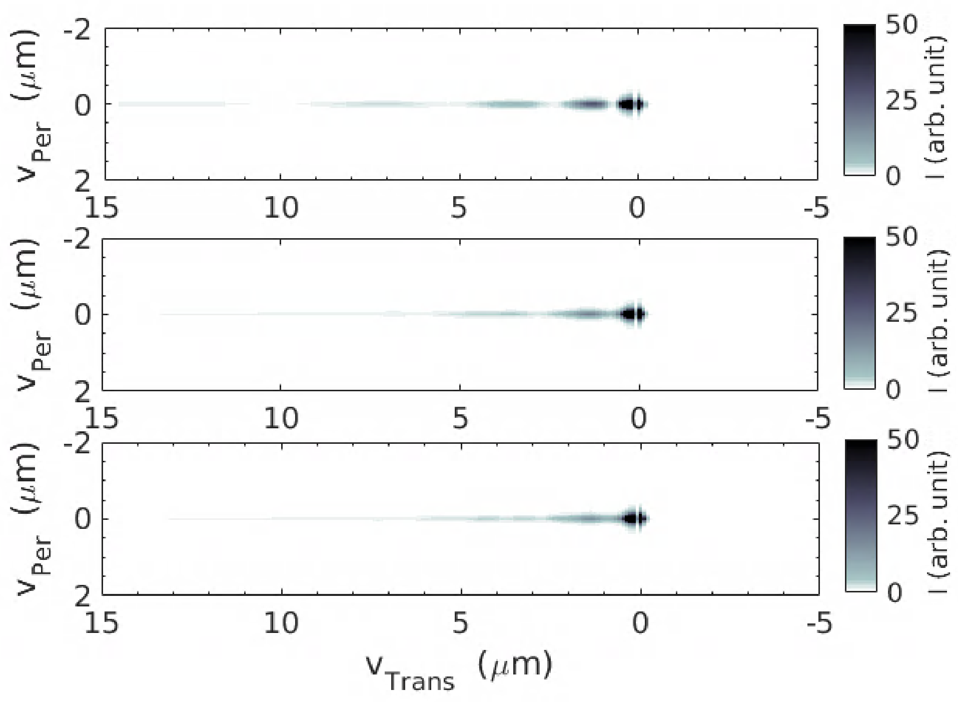


FIG. S10. Simulation in 2D of the wave-front produced by three different strain states of the sample. Strain field decays exponentially from the surface into the bulk with an amplitude of (top) $5\cdot 10^{-5}$ with decay of 2 µm (middle) $10^{-4}$ with decay of 7 µm and (bottom) $10^{-4}$ with decay of 10 µm.

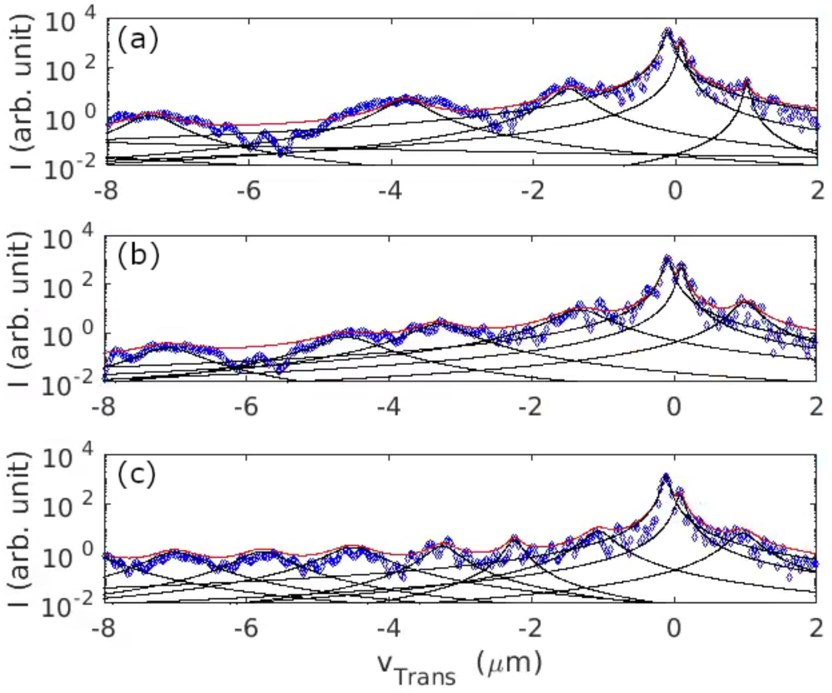


FIG. S11. (Blue dots) Line-cuts through the retrieved echoes from the indented Si sample in regions with different strain state, (black lines) representation of the different maxima using Lorentzian distributions. These were plotted using the values of intensity, width and location obtained with the Matlab function findpeaks on the retrieved data. (Red dash lines) Sum of the different Lorentzian functions to compare with the data collected. It is important to mention that the Lorenztian distribution does not properly represent the shape of the different maxima, and only a correct 3D model of the strain and of the dynamical diffraction process can be used to fit the data The echoes are not conventional diffraction peaks and one must think about them as constructive interference happening at the exit surface of the crystal. We only present the Lorentzian distributions for each maximum as a help to the reader. The order of the figures corresponds to the order presented in Fig. 3 of the main text.

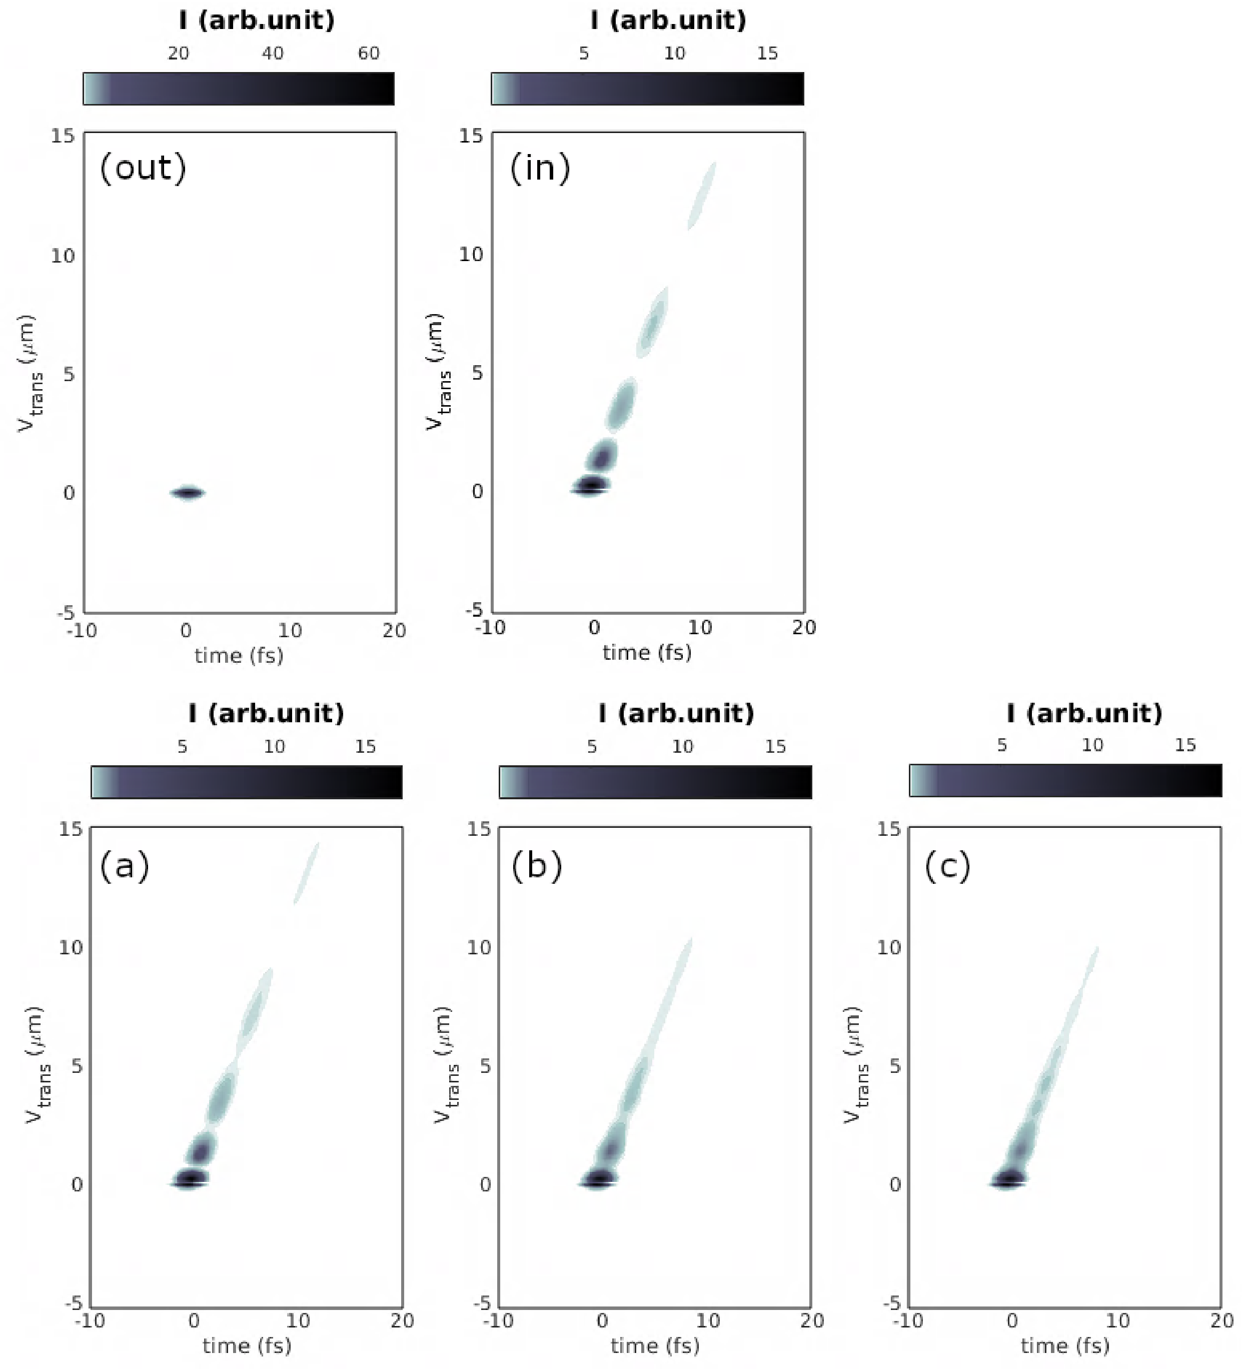


FIG. S12. Simulation of the relation between time delay and transverse displacement of the echoes for a Si 100 µm thick wafer at 8 keV without strain set to diffract horizontally ($\sigma - \pi$ scattering) to the (111) asymmetric Laue reflection at 8 keV. (top) Out and in the diffraction condition. (Bottom) in the diffraction condition for the three strain profiles comment in the main text (a), (b) and (c). The simulated temporal beam is a SASE like pulse with 2 fs FWHM and 1 eV energy bandwidth.

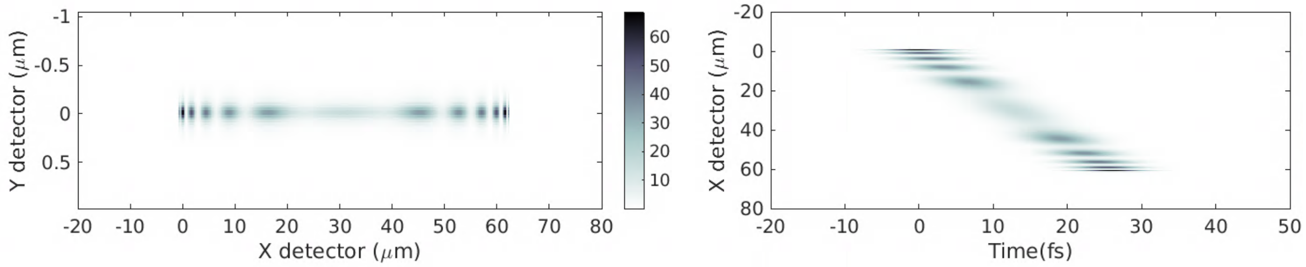


FIG. S13. Simulated signal in the diffraction direction for a Si 100 µm thick Si crystal at 8 keV for the (111) asymmetric horizontal Laue diffraction geometry. (Left) collected in a detector with nanometer resolution located at the focus of the beam and (right) conversion to time from the signal collected along the transverse direction to diffraction, assuming a incoming beam with 1 eV bandwidth and a temporal width of 2 fs

[1] P. F. Tavares et al., Commissioning and first-year operational results of the MAX IV 3 GeV ring, J. Synchrotron Rad. **25**, 1291 (2018).
[2] W. Decking et al., A MHz-repetition-rate hard x-ray free-electron laser driven by a superconducting linear accelerator, Nat. Photonics **14**, 391 (2020).
[3] J. M. Glownia et al., Time-resolved pump-probe experiments at the LCLS, Opt. Express **18**, 17620 (2010).
[4] U. Pietsch, V. Holy, and T. Baumbach, *High-Resolution X-Ray Scattering: From Thin Films to Lateral Nanostructures* (Springer-Verlad New York , LLC, 2004).
[5] P. Thibault, M. Dierolf, A. Menzel, O. Bunk, C. David, and F. Pfeiffer, High-resolution scanning x-ray diffraction microscopy, Science **321**, 379 (2008), https://science.sciencemag.org/content/321/5887/379.full.pdf.
[6] A. Ulvestad et al., Single Particle Nanomechanics in Operando Batteries via Lensless Strain Mapping, Nano Lett. **14**, 5123 (2014).
[7] A. Singer et al., Nucleation of dislocations and their dynamics in layered oxide cathode materials during battery charging, Nature Energy **3**, 641 (2018).
[8] P. Godard et al., Three-dimensional high-resolution quantitative microscopy of extended crystals, Nature Communications **2**, 568 (2011).
[9] M. O. Hill et al., Measuring three-dimensional strain and structural defects in a single InGaAs nanowire using coherent x-ray multiangle bragg projection ptychography, Nano Letters **18**, 811 (2018).
[10] S. O. Hruszkewycz et al., High-resolution three-dimensional structural microscopy by single-angle bragg ptychography, Nature Materials **16**, 244 (2017).
[11] V. Chamard, J. Stangl, G. Carbone, A. Diaz, G. Chen, C. Alfonso, C. Mocuta, and T. H. Metzger, Three-dimensional x-ray fourier transform holography: The bragg case, Phys. Rev. Lett. **104**, 165501 (2010).
[12] Q. Zhang, E. M. Dufresne, and A. R. Sandy, Dynamics in hard condensed matter probed by x-ray photon correlation spectroscopy: Present and beyond, Current Opinion in Solid State and Materials Science **22**, 202 (2018), advanced characterization of nanomaterials.
[13] V. Jacques, C. Laulhé, N. Moisan, S. Ravy, and D. Le Bolloc'h, Laser-induced charge-density-wave transient depinning in chromium, Phys. Rev. Lett. **117**, 156401 (2016).
[14] A. Schropp, P. Boye, J. M. Feldkamp, R. Hoppe, J. Patommel, D. Samberg, S. Stephan, K. Giewekemeyer, R. N. Wilke, T. Salditt, J. Gulden, A. P. Mancuso, I. A. Vartanyants, E. Weckert, S. Schöder, M. Burghammer, and C. G. Schroer, Hard x-ray nanobeam characterization by coherent diffraction microscopy, Applied Physics Letters **96**, 091102 (2010), https://doi.org/10.1063/1.3332591.
[15] J. Vila-Comamala, A. Diaz, M. Guizar-Sicairos, A. Mantion, C. M. Kewish, A. Menzel, O. Bunk, and C. David, Characterization of high-resolution diffractive x-ray optics by ptychographic coherent diffractive imaging, Opt. Express **19**, 21333 (2011).
[16] A. Schropp, R. Hoppe, V. Meier, J. Patommel, F. Seiboth, H. J. Lee, B. Nagler, E. C. Galtier, B. Arnold, U. Zastrau, J. B. Hastings, D. Nilsson, F. Uhlén, U. Vogt, H. M. Hertz, and C. G. Schroer, Full spatial characterization of a nanofocused x-ray free-electron laser beam by ptychographic imaging, Scientific Reports **3**, 1633 (2013).
[17] A. Björling et al., Ptychographic characterization of a coherent nanofocused X-ray beam, Opt. Express **28**, 5069 (2020).
[18] W. H. Zachariasen, *Theory of X-ray Diffraction in Crystals* (Dover Publications, INC, New York, 1945).
[19] B. Batterman and H. Cole, Dynamical diffraction of x-rays by perfect crystals, Reviews of Modern Physics **36**, 681 (1964).
[20] A. Authier, *Dynamical theory of X-ray diffraction* (Oxford University Press, 2001).
[21] J. Amann et al., Demonstration of self-seeding in a hard-x-ray free-electron laser, Nature Photonics **6**, 693 (2012).
[22] A. Pateras, J. Park, Y. Ahn, J. A. Tilka, M. V. Holt, H. Kim, L. J. Mawst, and P. G. Evans, Dynamical scattering in coherent hard x-ray nanobeam bragg diffraction, Phys. Rev. B **97**, 235414 (2018).
[23] M. Civita, A. Diaz, R. J. Bean, A. G. Shabalin, O. Y. Gorobtsov, I. A. Vartanyants, and I. K. Robinson, Phase modulation due to crystal diffraction by ptychographic imaging, Phys. Rev. B **97**, 104101 (2018).
[24] A. G. Shabalin, O. M. Yefanov, V. L. Nosik, V. A. Bushuev, and I. A. Vartanyants, Dynamical effects in bragg coherent x-ray diffraction imaging of finite crystals, Phys. Rev. B **96**, 064111 (2017).
[25] O. Y. Gorobtsov and I. A. Vartanyants, Phase of transmitted wave in dynamical theory and quasi-kinematical approximation, Phys. Rev. B **93**, 184107 (2016).
[26] Y. Shvydko and R. Lindberg, Spatiotemporal response of crystals in x-ray bragg diffraction, Phys. Rev. ST Accel. Beams **15**, 100702 (2012).
[27] A. Rodriguez-Fernandez et al., Spatial displacement of forward-diffracted x-ray beams by perfect crystals, Acta Cryst. A **74**, 75 (2018).
[28] A. Rodriguez-Fernandez et al., X-ray forward diffraction wave-front propagation in Si and C single crystals: simulations and experiments, Proc. of SPIE, Advances in Computational Methods for X-Ray Optics V, **11493**, 114930W (2020).
[29] E. H. R. Tsai, A. Diaz, A. Menzel, and M. Guizar-Sicairos, X-ray ptychography using a distant analyzer, Optics Express **24**, 6441 (2016).
[30] We note that conventional ptychography, in which the sample is scanned with respect to the incoming beam, would not work in presence of dynamical diffraction due the assumption of a factorization of the illumination and the sample transmissivity in conventional ptychography, ref. [5].
[31] M. Verezhak et al., Visualization of crystallographic defects in InSb micropillars by ptychographic topography, Microscopy

and Microanalysis **24**, 18 (2018).
[32] M. Verezhak, S. Van Petegem, A. Rodriguez-Fernandez, P. Godard, K. Wakonig, D. Karpov, V. L. R. Jacques, A. Menzel, L. Thilly, and A. Diaz, X-ray ptychographic topography: A robust nondestructive tool for strain imaging, Phys. Rev. B **103**, 144107 (2021).
[33] G. Batignani et al., Probing femtosecond lattice displacement upon photo-carrier generation in lead halide perovskite, Nature Communications **9**, 1971 (2018).
[34] Supplemental material. URL to be assigned (2020).
[35] C. Reuber, P. Eisenlohr, F. Roters, and D. Raabe, Dislocation density distribution around an indent in single-crystalline nickel: Comparing nonlocal crystal plasticity finite-element predictions with experiments., Acta Mareriala **71**, 333 (2014).
[36] M. Lie, C. Lu, K. Tieu, and H. Yu, Numereical comparison between berkovich and conical nano-indentations: Mechanical behaviour and micro-texture evolution, Materials Science & Engineering A **619**, 57 (2014).
[37] From Bragg's law $2d \sin\theta = n\lambda$.
[38] K. Wakonig et al., Ptychoshelves, a versatile highlevel framework for high-performance analysis of ptychographic data, Journal of applied crystallography **53**, 574 (2020).
[39] P. Thibault et al., Probe retrieval in ptychographic coherent diffractive imaging, Ultramicroscopy **109**, 338 (2009).
[40] P. Thibault and M. Guizar-Sicairos, Maximum-likelihood refinement for coherent diffractive imaging, New Journal of Physics **14** (2012).
[41] M. Guizar-Sicairos et al., High-throughput ptychography using eiger: scanning x-ray nano-imaging of extended regions, Optics Express **22**, 14859 (2014).
[42] M. van Heel and M. Schatz, Fourier shell correlation threshold criteria, Journal of Structural Biology **151**, 250 (2005).
[43] B. Lings et al., Simulations of time-resolved x-ray diffraction in laue geometry, J. Phys.: Condens. Matter **18**, 9231–9244 (2006).
[44] S. Takagi, Dynamical theory of diffaction applicable to cystals with any kind of small distortions, Acta. Cryst. **15**, 1311 (1962).
[45] N. Kato and A. R. Lang, A study of pendellösung fringes in x-ray diffraction, Acta Cryst. **12**, 787 (1959).
[46] Z. J. Li et al, Local strain and defects in silicon wafers due to nanoindentation revealed by full-field X-ray microdiffraction imaging, Journal of Synchrotron Radiation **22**, 1083 (2015).
